# Supplementary material for: Level Set Teleportation: An Optimization Perspective
Source: arXiv:2403.03362 source file (2025-03-18)
Supplement: Supplementary file 1 [file algorithm.tex]

Now we briefly discuss how to terminate our algorithm.
Suppose that \( \bar x \) is a local maximum of \cref{eq:sublevel-teleport}.
If the linear independence constraint qualification (LICQ) holds, 
then \( \bar x \) must satisfy the KKT conditions for some \( \lambda > 0 \)
\citep{bertsekas1997nonlinear},
\begin{align}\label{eq:kkt-conditions}
    \nabla^2 f(\xk) \grad(\xk) / \norm{\grad(\xk)} + \lambda \grad(\xk)
    &= 0,\\ 
    f(\xk) \leq f(\wk) \quad \text{and} \quad \lambda (f(\xk) - f(\wk)) &= 0. \nonumber
\end{align}
That is, \( \nabla^2 f(\xk) \grad(\xk) \propto \grad(\xk) \) and the 
sub-level set constraint is satisfied.
The teleportation problem satisfies LICQ unless \( \grad(\bar x) =
0 \); 
in this case, stationarity at \( \bar x \) implies stationarity over all of \(
\calS_k \) and teleporting is not interesting.
Thus, we assume LICQ holds and combine termination based on the KKT conditions
with line-search to give a complete solver in \cref{alg:teleport}.
